# Supplementary material for: Diffusion Models as Data Mining Tools
Source: arXiv:2408.02752 source file (2024-07-20)
Supplement: Supplementary file 1 [file finetuning-supmat.tex]

\begin{figure}[!ht]
    \centering
    \begin{subfigure}{0.43\textwidth}
        \centering
        \includegraphics[width=\textwidth]{operational-images-supmat/cars/pt/clusters/ranked/dift-161/32/1960__hard_limit_7__top_k_7__min_im_6.png}
        \includegraphics[width=\textwidth]{operational-images-supmat/faces/pt/clusters/random/dift-161/32/1880__hard_limit_7__top_k_7__min_im_6.png}
        \includegraphics[width=\textwidth]{operational-images-supmat/geo/pt/clusters/ranked/clip/32/Thailand__hard_limit_7__top_k_7__min_im_6.png}

        \caption{\textbf{Stable Diffusion (V1.5)}}
    \end{subfigure}
    \hspace{1em}
    \begin{subfigure}{0.43\textwidth}
        \centering
        \includegraphics[width=\textwidth]{operational-images-supmat/cars/ft/clusters/ranked/dift-161/32/1960__hard_limit_7__top_k_7__min_im_6.png}
        \includegraphics[width=\textwidth]{operational-images-supmat/faces/ft/clusters/ranked/dift-161/32/1880__hard_limit_7__top_k_7__min_im_6.png}
        \includegraphics[width=\textwidth]{operational-images-supmat/geo/ft/clusters/ranked/clip/32/Thailand__hard_limit_7__top_k_7__min_im_6.png}
        \caption{\textbf{Finetuned}}
    \end{subfigure}

    \caption{\textbf{Top-7 Cluster before and after finetuning}. We show results in 3 different datasets CarDB (1960) \cite{cardb}, FTT (1880) \cite{ftt}, and $G^3$ (Thailand) \cite{g3}. **See text for details.}
    \label{fig:finetuning-qualitative}
\end{figure}
